# Supplementary material for: Convolutional Conditional Neural Processes
Source: arXiv:2408.09583 source file (2024-08-18)
Supplement: Supplementary file 1 [file holder.tex]

\documentclass[12pt]{report}
\usepackage{libertine}

% General packages:
\usepackage[utf8]{inputenc}    % Input encoding
\usepackage[T1]{fontenc}       % Font encoding
\usepackage[british]{babel}    % Naming of figures and such
\usepackage[british]{isodate}  % Formatting of dates
\cleanlookdateon               % Show dates cleanly.
\usepackage{minted}            % Needs to be loaded before `csquotes`.
\usepackage[
    citestyle    = authoryear,
    bibstyle     = authoryear,
    giveninits   = true,
    uniquename   = init,
    uniquelist   = false,
    sortlocale   = en_GB,
    backend      = biber,
    backref      = true,
    maxbibnames  = 100,
    maxcitenames = 1,
    dashed       = false,
    % Needed to get sorting right for tussenvoegsels.
    %sortcites    = true,       
    ]{biblatex}                % Bibliography
\usepackage[
    style=american
    ]{csquotes}                % Required for BiBLaTeX
\usepackage{import}            % Importing subdocuments
\usepackage{standalone}        % Compilable subdocuments
% `setspace` needs to be loaded before `hyperref`.
\usepackage{setspace}          % Set line spacing
\usepackage{hyperref}          % Clickable references
\usepackage{microtype}         % Nice typography
\usepackage{makeidx}           % Make an index
\usepackage{silence}           % Silence warnings and errors
\WarningFilter{remreset}{The remreset package}
\WarningFilter*[parskip]{latex}{Command}

% Set line spacing.
\setstretch{1.25}

% Page layout:
\usepackage{tocloft}         % Control ToC
\usepackage[
    a4paper,
    bottom     = 1.1in,
    top        = 1.1in,
    left       = 1.1in,
    right      = 1.1in,
    headheight = 15pt,
    footskip   = 1.5\baselineskip
    ]{geometry}              % Margins
\usepackage{fancyhdr}        % Header
\usepackage{lastpage}        % Page numbers in footer
\usepackage{setspace}        % Line spacing
\usepackage{ragged2e}        % Better line endings
\ActivateWarningFilters[parskip]
\usepackage[
    parfill
    ]{parskip}               % Newlines instead of indentation
\DeactivateWarningFilters[parskip]
\usepackage{titlesec}        % Size of sections
\usepackage{titlecaps}       % Automatic capitalisation of titles
\usepackage[
    hang,
    bottom
    ]{footmisc}              % Configure footnotes
\usepackage{afterpage}       % Include stuff after the current page
\usepackage{placeins}        % Things like `\FloatBarrier`
\usepackage{pdflscape}       % Turn pages sideways
\usepackage{emptypage}       % Remove pagenumbers on empty pages

% Utility:
\usepackage[table]{xcolor}   % Colours
\usepackage[
    separate-uncertainty=true,
    per-mode=symbol
    ]{siunitx}               % Display units
\usepackage{enumitem}        % Better enumeration
\usepackage{xifthen}         % If statements
\usepackage{xpatch}          % Patch things
\usepackage{lipsum}          % Dummy text
\usepackage{listings}        % Listings
\usepackage{xparse}          % Better arguments for \newcommand
\usepackage{xfrac}           % Better fractions
\usepackage{etoolbox}        % Patch stuff
\usepackage[
    notquote
    ]{hanging}               % Hanging paragraphs
\usepackage{scalerel}        % Scale objects
\usepackage{soul}            % Highlighting

% Figures:
\usepackage{pgfplots}        % Plots
\pgfplotsset{compat=newest}
\usepackage{tikz}            % TikZ figures
\usepackage{float}           % Control floating of figures
\usepackage{multirow}        % Cells spanning multiple rows
\usepackage{graphicx}        % Graphics
\usepackage{caption}         % Subfigures and captions
\usepackage{subcaption}      % Subfigures and captions
\usepackage{booktabs}        % Nice looking tables
\usepackage{tabularx}        % Extended functionality for tables

% Math:
\usepackage{amsmath}         % Math
\usepackage{amssymb}         % Math symbols
\usepackage{mathtools}       % Math tools
\usepackage{amsthm}          % Theorems
\usepackage{thmtools}        % More math theorems
\usepackage{bm}              % Bold math symbols
\usepackage{bbm}             % More bold math symbols
\usepackage{cancel}          % Cancel equations
\usepackage{upgreek}         % Upright greek symbols
\usepackage[
    artemisia
    ]{textgreek}             % Greek symbols in text

% This package should be loaded last.
\usepackage[
    noabbrev,
    capitalize,
    nameinlink]{cleveref}    % Automatic referencing

% Add a comma in the cite style.

% Make sure that every `\citeyear` also prints the disambiguating `extradate`.
\DeclareCiteCommand{\citeyearlabel}
    {\usebibmacro{prenote}}
    {\printfield{year}\printfield{extradate}}
    {\multicitedelim}
    {\usebibmacro{postnote}}

\let\citeyear\citeyearlabel

% Define a standard for citing within theorem statements.

% Remove the colon after "In" in the bibliograhpy.
\renewbibmacro*{in:}{\bibstring{in} }

% Tune the electronic print field.
\DeclareFieldFormat{eprint}{%
  \iffieldundef{eprinttype}
    {Electronic print}
    {\thefield{eprinttype}}%
  \addcolon\space
  \ifhyperref
    {\url{#1}}
    {\nolinkurl{#1}}%
  \iffieldundef{eprintclass}
    {}
    {\addspace\mkbibparens{\thefield{eprintclass}}}\printtext{.}}

% Tune URL.
\DeclareFieldFormat{url}{\mkbibacro{URL}\addcolon\space\url{#1}\printtext{.}}

% Tune DOI.
\DeclareFieldFormat{doi}{%
  \mkbibacro{DOI}\addcolon\space
  \ifhyperref
    {\href{https://doi.org/#1}{\nolinkurl{#1}}}
    {\nolinkurl{#1}}\printtext{.}}

% In the below, we will redefine `\finentry` to not print a period if
%` pageref` exists. The period is then added back by `pageref`, but before the
% parentheses. Problems occur when `urldate` is also defined. In that case, 
% the extra period by `pageref` will add a period after `urldate`s
% parentheses, which we do not want. We use the toggle `printperiod` to detect
% this case.

% Tune "visited on".
\DeclareFieldFormat{urldate}{\mkbibparens{\bibstring{urlseen}\space#1\printtext{.}}}
\newtoggle{printperiod}
\toggletrue{printperiod}
\AtBeginBibliography{\renewbibmacro*{urldate}{\printurldate\togglefalse{printperiod}}}

% Tune "cited on".
\renewbibmacro*{finentry}{\iflistundef{pageref}{}{}\finentry}
\renewbibmacro*{pageref}{%
  \iflistundef{pageref}
    {}
    {\iftoggle{printperiod}{\setunit{\adddot\addspace}}{}\toggletrue{printperiod}\printtext[parens]{%
       \ifnumgreater{\value{pageref}}{1}
         {\bibstring{backrefpages}\ppspace}
         {\bibstring{backrefpage}\ppspace}%
          \printlist[pageref][-\value{listtotal}]{pageref}.}}}

% Add Oxford comma.
\DefineBibliographyExtras{british}{}

% Don't abbreviate the backreferences.
\DefineBibliographyStrings{english}{%
    backrefpage = {Cited on page},
    backrefpages = {Cited on pages}
}

% Get tussenvoegsels right. This is not a perfect solution, because the
% in-text citations will be sorted as if the tussenvoegsel is part of the
% last name.
\makeatletter
\AtBeginDocument{\toggletrue{blx@useprefix}}
\AtBeginBibliography{\togglefalse{blx@useprefix}}
\makeatother

% Make an index.
\makeindex

% Show the page number in the bottom center.
\fancypagestyle{plain}{
    \fancyhf{}                          % Clear all header and footers.
      % Remove the header rule.
    \cfoot{\thepage}                    % Show page number in the center.
}
\pagestyle{plain}

% Chapter styling from https://texblog.org/2012/07/03/fancy-latex-chapter-styles/
\newcommand{\hsp}{\hspace{20pt}}
\titleformat{\chapter}[hang]
    {\Huge\bfseries}
    {\thechapter\hsp\textcolor{gray75}{|}\hsp}
    {0pt}
    {\Huge\bfseries}
\titleformat{\section}
    {\normalfont\Large\bfseries\raggedright}
    {\thesection}
    {1em}
    {}
\titleformat{\subsection}
    {\normalfont\large\bfseries\raggedright}
    {\thesubsection}
    {1em}
    {}

% Set spacing after chapter equal to spacing right before section. Then
% things look nicely aligned.
\titlespacing{\chapter}{0pt}{3.5ex}{3.5ex}

% Define the styling of paragraphs.
\renewcommand{\paragraph}[1]{\textbf{#1.}}

% Redefine abstract environment.

% Kill any use of the \cite command.
\renewcommand{\cite}[1]{\PackageError{thesis}{use either parencite or authorcite}{}}

% Configure captions.
\WarningFilter{caption}{Unused \captionsetup}
\captionsetup[table]{font=small}
\captionsetup[figure]{font=small}

% Shortcuts for writing.

% \ifempty command:
\newcommand{\ifempty}[3]{\ifthenelse{\equal{#1}{}}{#2}{#3}}

% Style footnotes.
\setlength{\skip\footins}{\baselineskip}
\setlength{\footnotesep}{.75\baselineskip}

\setlength{\footnotemargin}{1em}

% Typewriter font:
  % Courier

% Define some colours.
\definecolor{darkblue} {rgb} {0.0 , 0.0 , 0.65}
\definecolor{darkred}  {rgb} {0.80, 0.0 , 0.0 }
\definecolor{redaccent}{HTML}{E64C66}
\definecolor{darkgreen}{rgb} {0.0 , 0.50, 0.0 }
\definecolor{gray75}   {gray}{0.75}

% Define shortcuts for colours.

% Use colours to define checkmarks and crosses.
\usepackage{pifont}

% Load TikZ libraries.
\usetikzlibrary{
    calc,
    positioning,
    fit,
    tikzmark,
    arrows.meta,
    shapes,
    decorations.pathreplacing,
    intersections,
    through
}
% Graphical models:
\tikzset{
    line/.style = {
        thick,
        ->,
        > = {
            Triangle[length=1.5mm, width=1.5mm]
        }
    },
    arrow/.style = {
        line
    },
    % Invisible node:
    hidden node/.style = {
        circle,
        minimum size = 1cm,
        draw = white,
        thick
    },
    % Latent variable:
    latent node/.style = {
        hidden node,
        draw = black,
    },
    % Latent variable:
    factor node/.style = {
        hidden node,
        rectangle,
        draw = black,
    },
    % Observed variable:
    observed node/.style = {
        latent node,
        fill = gray!15
    },
    % Plate:
    plate/.style = {
        draw,
        label={[anchor=north west]south west:#1},
        rounded corners=2pt,
        shape=rectangle,
        inner sep=10pt,
        thick
    }
}

% Circled number:

% Style enumerate and lists. Do not use `label=(\arabic*)` because equation
% numbering already uses the same style.
\setenumerate{topsep=.25\baselineskip, itemsep=0pt}
\setlist{topsep=.25\baselineskip, itemsep=0pt}
% \setlist[enumerate]{
%     label=(\arabic*),
%     itemsep=-0.25\baselineskip,
%     topsep=0.25\baselineskip,
%     after={\vspace*{0.25\baselineskip}}
% }
% \setlist[enumerate,2]{
%     topsep=-0.25\baselineskip,
%     itemsep=0pt,
%     label=(\alph*)
% }
% \setlist[enumerate,3]{
%     topsep=-0.25\baselineskip,
%     itemsep=0pt,
%     label=(\roman*)
% }
% \setlist[itemize]{
%     label=\textbullet,
%     itemsep=-0.25\baselineskip,
%     topsep=0.25\baselineskip
% }
% \setlist[itemize,2]{
%     topsep=-0.25\baselineskip,
%     itemsep=0pt
% }
% \setlist[itemize,3]{
%     topsep=-0.25\baselineskip,
%     itemsep=0pt
% }

% Set the default float placement correctly.
\floatplacement{figure}{tbp}
\floatplacement{table}{tbp}

% Set spacing between figures and text.
\setlength{\textfloatsep}{30pt plus 1.0pt minus 2.0pt}
\setlength{\floatsep}{30pt plus 1.0pt minus 2.0pt}
\setlength{\intextsep}{30pt plus 1.0pt minus 2.0pt}

% Adjust line spacing in captions.
\captionsetup{font={stretch=1.25}}

% Newline for in a title.

% Define outline tools.

\newlist{outlinelist}{enumerate}{1}
\setlist[outlinelist]{
    label=\arabic*.,
    noitemsep,
    topsep=0pt,
    parsep=0pt,
    partopsep=0pt
}
\newcommand{\note}[1]{{\color{darkred}#1}}

% Left-justified text in tabularx environment:
\newcolumntype{L}{>{\RaggedRight\arraybackslash}X}

% Hyperlink setup.
\hypersetup{
    colorlinks,
    citecolor = black,
    filecolor = black,
    linkcolor = black,
    urlcolor  = black
}

% Landscape figures:

% Hanging full citation:

\input{preamble/math}
  % We'll configure our own numbering below.
% Patch \listoftheorems.
%   Source: https://tex.stackexchange.com/questions/249963/remove-repeated-theorem-in-the-list-of-theorems
\makeatletter
\patchcmd\thmt@mklistcmd
    {\thmt@thmname}
    {\check@optarg{\thmt@thmname}}
    {}{}
\patchcmd\thmt@mklistcmd
    {\thmt@thmname\ifx}
    {\check@optarg{\thmt@thmname}\ifx}
    {}{}
\protected\def\check@optarg#1{%
    \@ifnextchar\thmtformatoptarg\@secondoftwo{#1}%
}
\makeatother

% Define lists of things commands.
\let\oldlistoftheorems\listoftheorems

\renewcommand{\listoftheorems}{
    \renewcommand{\listtheoremname}{List of Theorems}
    \oldlistoftheorems[ignoreall, show={theorem}]
}

% Define environments.
\newlength{\thmtopsep}\setlength{\thmtopsep}{\topsep}
\newlength{\thmbotsep}\setlength{\thmbotsep}{\topsep}
\newtheoremstyle{theoremstyle}
    {\thmtopsep}{\thmbotsep}
    {}           % Body font
    {}           % Indent amount
    {\bfseries}  % Theorem head font
    {.}          % Punctuation after theorem head
    {.5em}       % Space after theorem head
    {}           % Theorem head spec
\theoremstyle{theoremstyle}

\ifcsname notheorems\endcsname
\else
    \newtheorem{theorem}{Theorem}[section]
    \newtheorem{proposition}{Proposition}[section]
    \newtheorem{corollary}{Corollary}[section]
    \newtheorem{fact}{Fact}[section]
    \newtheorem{lemma}{Lemma}[section]

    \newtheorem{assumption}{Assumption}[section]
    \newtheorem{definition}{Definition}[section]
    \newtheorem{question}{Question}[section]
    \newtheorem{example}{Example}[section]
    \newtheorem{model}{Model}[section]
    \newtheorem{remark}{Remark}[section]
\fi

% Set referencing formats.
\crefname{assumption}{Assumption}{Assumptions}
\Crefname{assumption}{Assumption}{Assumptions}
\crefname{corollary}{Corollary}{Corollaries}
\Crefname{corollary}{Corollary}{Corollaries}
\crefname{definition}{Definition}{Definitions}
\Crefname{definition}{Definition}{Definitions}
\crefname{example}{Example}{Examples}
\Crefname{example}{Example}{Examples}
\crefname{fact}{Fact}{Facts}
\Crefname{fact}{Fact}{Facts}
\crefname{lemma}{Lemma}{Lemmas}
\Crefname{lemma}{Lemma}{Lemmas}
\crefname{model}{Model}{Models}
\Crefname{model}{Model}{Models}
\crefname{proposition}{Proposition}{Propositions}
\Crefname{proposition}{Proposition}{Propositions}
\crefname{question}{Question}{Questions}
\Crefname{question}{Question}{Questions}
\crefname{remark}{Remark}{Remarks}
\Crefname{remark}{Remark}{Remarks}
\crefname{theorem}{Theorem}{Theorems}
\Crefname{theorem}{Theorem}{Theorems}

% Referentiable list items in environments
\newlist{asslist}{enumerate}{1}
\setlist[asslist]{
    ref=\theassumption.(\arabic*),
    label=(\arabic*),
    % topsep=0pt,
}
\crefname{asslisti}{Assumption}{Assumptions}
\Crefname{asslisti}{Assumption}{Assumptions}
\newlist{corlist}{enumerate}{1}
\setlist[corlist]{
    ref=\thecorollary.(\arabic*),
    label=(\arabic*),
    % topsep=0pt,
}
\crefname{corlisti}{Corollary}{Corollaries}
\Crefname{corlisti}{Corollary}{Corollaries}
\newlist{deflist}{enumerate}{1}
\setlist[deflist]{
    ref=\thedefinition.(\arabic*),
    label=(\arabic*),
    % topsep=0pt,
}
\crefname{deflisti}{Definition}{Definitions}
\Crefname{deflisti}{Definition}{Definitions}
\newlist{exlist}{enumerate}{1}
\setlist[exlist]{
    ref=\theexample.(\arabic*),
    label=(\arabic*),
    % topsep=0pt,
}
\crefname{exlisti}{Example}{Examples}
\Crefname{exlisti}{Example}{Examples}
\newlist{factlist}{enumerate}{1}
\setlist[factlist]{
    ref=\thefact.(\arabic*),
    label=(\arabic*),
    % topsep=0pt,
}
\crefname{factlisti}{Fact}{Facts}
\Crefname{factlisti}{Fact}{Facts}
\newlist{lemlist}{enumerate}{1}
\setlist[lemlist]{
    ref=\thelemma.(\arabic*),
    label=(\arabic*),
    % topsep=0pt,
}
\crefname{lemlisti}{Lemma}{Lemmas}
\Crefname{lemlisti}{Lemma}{Lemmas}
\newlist{modlist}{enumerate}{1}
\setlist[modlist]{
    ref=\themodel.(\arabic*),
    label=(\arabic*),
    % topsep=0pt,
}
\crefname{modlisti}{Model}{Models}
\Crefname{modlisti}{Model}{Models}
\newlist{proplist}{enumerate}{1}
\setlist[proplist]{
    ref=\theproposition.(\arabic*),
    label=(\arabic*),
    % topsep=0pt,
}
\crefname{proplisti}{Proposition}{Propositions}
\Crefname{proplisti}{Proposition}{Propositions}
\newlist{qlist}{enumerate}{1}
\setlist[qlist]{
    ref=\theremark.(\arabic*),
    label=(\arabic*),
    % topsep=0pt,
}
\crefname{qlisti}{Question}{Questions}
\Crefname{qlisti}{Question}{Questions}
\newlist{remlist}{enumerate}{1}
\setlist[remlist]{
    ref=\theremark.(\arabic*),
    label=(\arabic*),
    % topsep=0pt,
}
\crefname{remlisti}{Remark}{Remarks}
\Crefname{remlisti}{Remark}{Remarks}
\newlist{thmlist}{enumerate}{1}
\setlist[thmlist]{
    ref=\thetheorem.(\arabic*),
    label=(\arabic*),
    % topsep=0pt,
}
\crefname{thmlisti}{Theorem}{Theorems}
\Crefname{thmlisti}{Theorem}{Theorems}

% Reference numbers in the list.

% Backward compatibility:

% We actually will use coloured links.
\definecolor{aquamarine}{HTML}{218274}
\hypersetup{
    colorlinks,
    citecolor = aquamarine,
    filecolor = aquamarine,
    linkcolor = aquamarine,
    urlcolor  = aquamarine,
}

% Use italic font in bodies for clarity.
\newtheoremstyle{theoremstyle}
    {\thmtopsep}{\thmbotsep}
    {\itshape}   % Body font
    {}           % Indent amount
    {\bfseries}  % Theorem head font
    {.}          % Punctuation after theorem head
    {.5em}       % Space after theorem head
    {}           % Theorem head spec
\theoremstyle{theoremstyle}

% Set numbering of theorems right.
\newtheorem{theorem}{Theorem}[chapter]
\newtheorem{proposition}[theorem]{Proposition}

\newtheorem{lemma}[theorem]{Lemma}

% Hack `\listoftheorem` to remove the title.
\makeatletter
\renewcommand\listoftheorems[1][]{%
    \begingroup
    \setlisttheoremstyle{#1}%
    \let\listfigurename\listtheoremname
    \def\contentsline##1{%
        \csname thmt@contentsline@##1\endcsname{##1}%
    }%
    \@for\thmt@envname:=\thmt@allenvs\do{%
        \thmtlo@newentry
    }%
    \let\thref@starttoc\@starttoc
    \def\@starttoc##1{\thref@starttoc{loe}}%
    \@fileswfalse
    \AtEndDocument{%
        \if@filesw
        \@ifundefined{tf@loe}{%
            \expandafter\newwrite\csname tf@loe\endcsname
            \immediate\openout \csname tf@loe\endcsname \jobname.loe\relax
        }{}%
        \fi
    }%
    \@starttoc{lof}
    \endgroup
}
\makeatother

% Fix spacing around proofs.
\xpatchcmd{\proof}{\topsep6\p@\@plus6\p@\relax}{}{}{}
\BeforeBeginEnvironment{proof}{\vspace{-0.5em}}
\AfterEndEnvironment{proof}{\vspace{-0.5em}}

% Commands specific for thesis:

% Listings:
\usepackage{tcolorbox}
\tcbuselibrary{minted,skins,breakable}

\definecolor{solarized-light-bg}{HTML}{fdf6e3}
\definecolor{solarized-light-fg}{HTML}{586e75}
\newtcblisting{pythoncode}[2]{
    listing engine = minted,
    listing only,
    minted style = solarized-light,
    minted language = python,
    minted options = {
        fontsize = #1,
        escapeinside = ||,
        mathescape = true,
        highlightlines = #2,
        highlightcolor = red,
    },
    colback = solarized-light-bg,
    colframe = solarized-light-bg,
    toprule = 0pt,
    left = 5pt,
    left = 5pt,
    leftrule = 0pt,
    rightrule = 0pt,
    bottomrule = 0pt,
    arc = 0pt,
    frame hidden,
    breakable,
}
% Disable italics.
\AtBeginEnvironment{pythoncode}{\let\itshape\relax}

% Override the textwriter font.
%\usepackage[scaled=0.8]{beramono}
\usepackage[scaled=0.95]{inconsolata}

% We never want footnotes to break across pages.
\interfootnotelinepenalty=10000

% Allow restatable environments.

\newcommand{\statement}[1]{
    \begingroup
        \subimport{}{#1}
        \ifempty{\statementoption}{
            \csname\statementtype\endcsname
        }{
            \expandafter\csname\statementtype\endcsname[\statementoption]%
        }
        \label{\statementlabel}
        \statementcontent
        \csname end\statementtype\endcsname
    \endgroup
}

\addbibresource{../../bibliography.bib}

\begin{document}

\chapter{\texorpdfstring{$L^p$-$\beta$}{Lp-beta}-H\"older Equicontinuity}
\label{chap:holder}

\section{Weak Convergence}
Let $(\mu_i)_{i=1}^\infty \sub \mathcal{P}$ and $\mu \in \mathcal{P}$.
We say that $\mu_i$ converges weakly to $\mu$ and write $\mu_i \weakto \mu$ if $\mu_i(L) \to \mu(L)$ for all continuous bounded functions $L\colon C(\mathcal{X}, \mathcal{Y}) \to \R$.
Consider the natural embedding $\iota_R \colon C(\mathcal{X}, \mathcal{Y}) \to C([-R, R], \mathcal{Y})$ and denote $\mu|_{[-R, R]} = \iota_R(\mu)$.
The following proposition allows us to deduce weak convergence from weak convergence on all compacts.

\begin{proposition} \label{prop:weak_convergence_from_compacts}
    $\mu_i \weakto \mu$ if and only if $\mu_i|_{[-R,R]} \weakto \mu|_{[-R, R]}$ for all $R > 0$.
\end{proposition}

\begin{proof}
    Let $L\colon C(\mathcal{X}, \mathcal{Y}) \to \R$ be continuous and bounded.
    Let $R > 0$.
    Consider the particular right inverse $\iota_R^\dagger \colon C([-R, R], \mathcal{Y}) \to C(\mathcal{X}, \mathcal{Y})$ of $\iota_R$ defined by $\iota_R^\dagger(f)(x) = f(\sign(x)(\abs{x} \land R))$.
    By construction of $d_C$, we can find $\e > 0$ such that, for all $f, g \in C(\mathcal{X}, \mathcal{Y})$, we have $\abs{L(f) - L(g)} < \e$ whenever $g|_{[-R, R]} = f|_{[-R, R]}$.
    Therefore,
    \begin{equation}
        \sup_{i \ge 1}\,
        \abs{
            \E_{\mu_i\cond_{[-R, R]}}[L \comp \iota_R^\dagger(f)] -
            \E_{\mu_i}[L(f)]
        }
        \le
        \sup_{i \ge 1}\,
        \E_{\mu_i}[\abs{
            L(\iota_R^\dagger \comp \iota_R(f)) -
            L(f)
        }]
        \le \e,
    \end{equation}
    because $\iota_R^\dagger \comp \iota_R(f)|_{[-R, R]} = f_{[-R, R]}$.
    In other words,
    \begin{equation}
        \lim_{R \to \infty} \E_{\mu_i\cond_{[-R, R]}}[L \comp \iota_R^\dagger(f)] = \E_{\mu_i}[L(f)] \quad \text{uniformly over $i \ge 1$}.
    \end{equation}
    Then compute
    \begin{align*}
        \lim_{i \to \infty} \E_{\mu_i}[L(f)]
        &= \lim_{i \to \infty} \lim_{R \to \infty} \E_{\mu_i|_{[-R, R]}}[L \comp \iota_R^\dagger(f)] \\
        &=  \lim_{R \to \infty} \lim_{i \to \infty} \E_{\mu_i|_{[-R, R]}}[L \comp \iota_R^\dagger(f)] \\
        &=  \lim_{R \to \infty} \E_{\mu|{[-R, R]}}[L \comp \iota_R^\dagger(f)] \\
        &= \E_{\mu}[L(f)]
    \end{align*}
    where the interchange of limits is justified by the aforementioned uniformity of convergence.
    Since $L$ was arbitrary, this shows that $\mu_i \weakto \mu$.
\end{proof}

\section{\texorpdfstring{$L^{p,q}$}{Lpq}-H\"older Equicontinuity}

We will want to deduce weak convergence from weak convergence of the finite-dimensional distributions.
For this, we define the notion of \emph{$L^{p,q}$-H\"older equicontinuity}.
Let $\mu \in \mathcal{P}$.
Call a single measure $\mu$ \emph{$L^{p,q}$-H\"older continuous} for some $p > 0$ and $q > 0$ if there exist a constant $c > 0$ and a radius $r > 0$ such that
\begin{equation}
    \E_\mu[\abs{f(x) - f(y)}^p] \le c \abs{x - y}^q
    \quad\text{whenever}\quad
    \abs{x - y} < r.
\end{equation}
Let $\mathcal{F} \sub \mathcal{P}$ be a family of probability measures.
Call this family \emph{$L^{p,q}$-H\"older equicontinuous} if there exist a constant $c > 0$ and a radius $r > 0$ such that
\begin{equation}
    \sup_{\mu \in \mathcal{F}}\,
    \E_\mu[\abs{f(x) - f(y)}^p] \le c \abs{x - y}^q
    \quad\text{whenever}\quad
    \abs{x - y} < r.
\end{equation}
This can also be written as a limit:
\begin{equation}
    \lim_{h \to 0}\,
    \sup_{\mu \in \mathcal{F}}\,
    \sup_{x \in \X}\,
    \frac{\E_\mu[\abs{f(x + h) - f(x)}^p]}{h^q}
    < \infty.
\end{equation}
If $\F$ are Gaussian processes, then the criterion simplifies.

\begin{proposition} \label{prop:Holder_continuity_Gaussians}
    Let $\F\ss{G} \sub \mathcal{P}\ss{G}$ be a family of non-degenerate Gaussian processes.
    For $\mu \in \F\ss{G}$, denote its mean function by $m_\mu\colon \mathcal{X} \to \R$ and its covariance function by $k_\mu\colon \X \times \X \to \R$.
    Let $p \ge 2$.
    Then $\F\ss{G}$ is $L^{p, q}$-H\"older equicontinuous if \note{[and only if?]} it is $L^{2, 2q/p}$-H\"older equicontinuous:
    \begin{align*}
        &\lim_{h \to 0}\,
        \sup_{\mu \in \F}\,
        \sup_{x \in \X}\,
        \frac{(m_\mu(x + h) - m_\mu(x))^2 + \Delta k_\mu(x + h, x)}{h^{2q/p}} \\
        &\qquad =
        \lim_{h \to 0}\,
        \sup_{\mu \in \F}\,
        \sup_{x \in \X}\,
        \frac{\E_\mu[\abs{f(x + h) - f(x)}^2]}{h^{2q/p}}
        < \infty
    \end{align*}
    where
    \begin{equation}
        \Delta k_\mu(x + h, x)
        = k_\mu(x + h, x + h) + k_\mu(x, x) - 2 k_\mu(x + h, x).
    \end{equation}
    Consequently, if $\F\ss{G}$ is $L^{p,q}$-H\"older equicontinuous for $p \ge 2$ if and only if $\F\ss{G}$ is $L^{\alpha p,\alpha q}$-H\"older equicontinuous with $\alpha > 0$ for $\alpha p \ge 2$.
\end{proposition}
\begin{proof}
    Note that
    \begin{equation}
        f(x + h) - f(x)
        \sim \Normal(m_\mu(x + h) - m_\mu(x), \Delta k_\mu(x + h, x)).
    \end{equation}
    For any $U \sim \Normal(\mu, \sigma^2)$, it holds that
    \begin{equation}
        \E[\abs{U}^p]
        \le 2^{p} M_p (\abs{\mu}^p + \sigma^{p})
    \end{equation}
    where $M_p = \E[\abs{N}^p] < \infty$ with $N \sim \Normal(0, 1)$.
    Therefore,
    \begin{equation}
        \frac{\E_\mu[\abs{f(x + h) - f(x)}^p]}{h^q}
        \le
        2^p M_p \frac{((m_\mu(x + h) - m_\mu(x))^2)^{p/2} + (\Delta k_\mu(x + h, x))^{p/2}}{h^q}.
    \end{equation}
    Since $p \ge 2$, $a^{p/2} + b^{p/2} \le (a + b)^{p/2}$ for $a, b \ge 0$, so
    \begin{equation}
        \frac{\E_\mu[\abs{f(x + h) - f(x)}^p]}{h^q}
        \le
        2 M_p\frac{ ((m_\mu(x + h) - m_\mu(x))^2 + \Delta k_\mu(x + h, x))^{p/2}}{h^q}.
    \end{equation}
    Hence, it is sufficient that
    \begin{equation}
        \lim_{h \to 0}\,
        \sup_{\mu \in \F}\,
        \sup_{x \in \X}\,
        2^p M_p
        \frac{((m_\mu(x + h) - m_\mu(x))^2 + \Delta k_\mu(x + h, x))^{p/2}}{h^q}
        < \infty.
    \end{equation}
    Equivalently, it is sufficient that
    \begin{equation}
        \lim_{h \to 0}\,
        \sup_{\mu \in \F}\,
        \sup_{x \in \X}\,
        \frac{(m_\mu(x + h) - m_\mu(x))^2 + \Delta k_\mu(x + h, x)}{h^{2q/p}}
        < \infty.
    \end{equation}
    Here the numerator is equal to $\E_\mu[\abs{f(x + h) - f(x)}^2]$, so we can also write
    \begin{equation}
        \lim_{h \to 0}\,
        \sup_{\mu \in \F}\,
        \sup_{x \in \X}\,
        \frac{\E_\mu[\abs{f(x + h) - f(x)}^2]}{h^{2q/p}}
        < \infty,
    \end{equation}
    which concludes the proof.
\end{proof}

If the Gaussian processes in $\F\ss{G}$ are stationary, then the condition simplifies to
\begin{equation}
    \lim_{h \to 0}\,
    \sup_{\mu \in \F\ss{G}}\,
    \frac{
        k_\mu(0)
        - k_\mu(h)
    }{h^{2q/p}}
    = 0.
\end{equation}
If the kernels are once differentiable at the origin, then, upon choosing $p = 4$ and $1 < q < 2$, it suffices that $\sup_{\mu \in \F\ss{G}} \norm{k'_\mu}_\infty < \infty$.
For kernels of the form $k_\mu(h) = \exp(-g_\mu(h))$ with $g(0) = 0$ where $g \colon [0, \infty) \to [0, \infty)$ is strictly increasing, we require \note{[double check this!]}
\begin{equation}
    \lim_{h \to 0}\,
    \sup_{\mu \in \F\ss{G}}\,
    \frac{
        g_\mu(h)
    }{h^{2q/p}}
    = 0.
\end{equation}
For example, if $g_\mu(h) = c_\mu h$ for $c_\mu > 0$, then, upon choosing $p = 4$ and $1 < q < 2$, it suffices that $\sup_{\mu \in \F\ss{G}}\, c_\mu < \infty$.

Let $I = \union_{n=1}^\infty \mathcal{X}^n$ denote the collection of all finite index sets.
For $\vx \in \R^n$, let $P_\vx\colon C(\mathcal{X}, \mathcal{Y}) \to \mathcal{Y}^n$ be the projection onto the index set $\vx$: $P_\vx f = (f(x_1), \ldots, f(x_n))$.
For $\vx \in \R^n$ and a measure $\mu \in \mathcal{P}$, let $P_\vx \mu$ be the corresponding pushforward measure.

\begin{lemma} \label{lem:modulus_continuity}
    Suppose that $(\mu_i)_{i=1}^\infty \sub \mathcal{P}$ are H\"older $L^{p,q}$-equicontinuous for some $p > 0$ and $q > 1$;
    that is, there exist $p > 0$, $q > 1$, a constant $c > 0$, and a radius $r > 0$ such that
    \begin{equation}
        \sup_{i \ge 1}\,
        \E_{\mu_i}[\abs{f(x) - f(y)}^p] \le c \abs{x - y}^q
        \quad\text{whenever}\quad
        \abs{x - y} < r.
    \end{equation}
    For $f \in C([0, 1], \Y)$, define the \emph{modulus of continuity} by
    \begin{equation}
        \omega_f(h)
        = \sup_{x, y \in [0, 1]: \abs{x - y} < h} \abs{f(x) - f(y)}.
    \end{equation}
    Then, for all $\e > 0$,
    \begin{equation}
        \lim_{h \to 0} \sup_{i \ge 1}\, \mu_i(\omega_f(h) \ge \e) = 0.
    \end{equation}
\end{lemma}
\begin{proof}
    Choose $k \in \N$ such that $2^{-(k + 1)} \le h \le 2^{-k}$.
    The proof strategy mimics the proof of Theorem 4.2.1 by \textcite{Norris:2018:Advanced_Probability}.
    Let $i \in \N$.
    For $n \in \N$, denote $\Db_n = \set{0, 2^{-n}, 2 \cdot 2^{-n}, \ldots, 1}$.
    Consider $f \in C([0, 1], \mathcal{Y})$.
    Set
    \begin{equation}
        K_n = \sup_{x \in \Db_n \setminus \set{1}} = \abs{f(x + 2^{-n}) - f(x)}.
    \end{equation}
    Overestimate the supremum by a sum and use $L^{p,q}$-H\"older continuity of $\mu_i$:
    \begin{equation}
         \E_{\mu_i}[K_n^p]
         \le \sum_{i=0}^{2^n - 1} \E_{\mu_i}[\abs{f(x + 2^{-n}) - f(x)}^p]
         \le \sum_{i=0}^{2^n - 1} 2^{-q n}
         = 2^{-(q - 1) n}.
    \end{equation}
    For any $x, y \in \union_{n=1}^\infty \Db_n$ such that $x < y < x + 2^{-k}$, note that the interval $[x, y)$ is the finite, disjoint union of intervals $[r, r + 2^{-n})$ with $r \in \Db_n$ for $n \ge k + 1$ where no three intervals have the same length.
    Therefore, for such $x$ and $y$, by continuity of $f$,
    \begin{equation}
        \omega_f(2^{-k})
        = \sup_{x, y \in \union_{n=1}^\infty \Db_n: \abs{x - y}< 2^{-k}}\abs{f(x) - f(y)}
        \le 2\sum_{n=k+1}^\infty K_n.
    \end{equation}
    Hence,
    \begin{equation}
        \E_{\mu_i}\sbrac{\omega_f(2^{-k})}
        % \le 2\sum_{n=k+1}^\infty \E_{\mu_i}[K_n]
        \le 2\sum_{n=k+1}^\infty \E_{\mu_i}[K_n^p]^{\frac1p}
        \le 2\sum_{n=k+1}^\infty 2^{-\frac{q - 1}{p}n}
        = \frac{2^{1-\frac{q - 1}{p}(k + 1)}}{1 - 2^{-\frac{q - 1}{p}}}
        = c_{p,q} 2^{-\frac{q - 1}{p}k},
    \end{equation}
    for some constant $c_{p, q}$ that depends on $p$ and $q$, using that $q > 1$.
    Then, for any $\e > 0$, by Markov's Inequality,
    \begin{equation}
        \sup_{i \ge 1}\, \mu_i(\omega_f(h) \ge \e)
        \le \sup_{i \ge 1}\, \mu_i(\omega_f(2^{-k}) \ge \e)
        \le \frac{c_{p,q}}{\e} 2^{-\frac{q - 1}{p}k}.
    \end{equation}
    This proves the result, because $k \to \infty$ as $h \to 0$.
\end{proof}

\begin{proposition} \label{prop:weak_convergence_from_fdds}
    Let $(\mu_i)_{i=1}^\infty \sub \mathcal{P}$ be weakly convergent to some $\mu \in \mathcal{P}$ along a dense sequence of finite-dimensional distributions: $P_{\vx_k} \mu_i \weakto P_{\vx_k} \mu$ for all $k \ge 1$ where $(\vx_k)_{k \ge 1} \sub I$ is a sequence that becomes dense in $\X$.
    If $(\mu_i)_{i=1}^\infty$ are H\"older $L^{p,q}$-equicontinuous for some $p > 0$ and $q > 1$, then $\mu_i \weakto \mu$.
\end{proposition}
\begin{proof}
    We demonstrate that $\mu_i|_{[-R, R]} \weakto \mu|_{[-R, R]}$ for all $R > 0$ and appeal to \cref{prop:weak_convergence_from_compacts}.
    For notational convenience, we only consider the restriction to $[0, 1]$ and suppress the notation for the restriction.

    For $\vx \in [0, 1]^n$, consider the particular right inverse $P_\vx^\dagger \colon \R^n \to C([0, 1], \mathcal{Y})$ of $P_\vx$ defined by setting $P_\vx^\dagger \vy$ to the linear interpolation through the points $(x_1,y_1), \ldots, (x_n, y_n)$ and letting it be constant outside the extremal inputs.
    Denote $\norm{f - g}_\infty = \sup_{x\in [0, 1]} \abs{f(x) - g(x)}$.

    The restriction $(\vx_k)_{k = 1}^\infty \sub \union_{n=1}^\infty [0, 1]^n$ becomes dense in $[0, 1]$.
    Therefore, by \cref{lem:modulus_continuity}, for every $\delta > 0$,
    \begin{equation}
        \lim_{k \to \infty} \sup_{i \ge 1}\, \mu_i(\norm{P_{\vx_k}^\dagger P_{\vx_k} f - f}_\infty \ge \delta) = 0.
    \end{equation}
    Note that we also have
    \begin{equation}
        \lim_{k \to \infty} \mu(\norm{P_{\vx_k}^\dagger P_{\vx_k} f - f}_\infty \ge \delta) = 0.
    \end{equation}
    This is because, $\mu$--almost surely, $f$ is continuous on a compact set, hence uniformly continuous, so $\norm{P_{\vx_k}^\dagger P_{\vx_k} f - f}_\infty \to 0$ almost surely and consequently in probability.

    Let $L\colon C([0, 1], \mathcal{Y}) \to \R$ be continuous and bounded.
    Let $\e > 0$.
    By continuity of $L$, there exists a $\delta > 0$ such that $\norm{f - g}_\infty < \delta$ implies that $\norm{L(f) - L(g)}_\infty < \e$.
    Consider the event $A^k_\delta = \set{\norm{P_{\vx_k}^\dagger P_{\vx_k} f - f} < \delta}$.
    Then estimate
    \begin{equation}
        \abs{
            \E_{\mu_i}[L(P_{\vx_k}^\dagger P_{\vx_k} f)]
            - \E_{\mu_i}[L(f)]
        }
        \le \e + \norm{L}_\infty \mu_i((A^k_\delta)^\c)
        \le \e + \norm{L}_\infty \sup_{i \ge 1} \,\mu_i((A^k_\delta)^\c).
    \end{equation}
    Therefore, taking $k \to \infty$ shows that
    \begin{equation}
        \lim_{k \to \infty} \E_{P_{\vx_k} \mu_i}[L \comp P_{\vx_k}^\dagger]
        = \E_{\mu_i}[L] \quad \text{uniformly over $i \ge 1$}.
    \end{equation}
    Moreover, the same limit holds for $\mu$.
    Then compute
    \begin{align*}
        \lim_{i \to \infty} \E_{\mu_i}[L]
        &= \lim_{i \to \infty} \lim_{k \to \infty} \E_{P_{\vx_k} \mu_i}[L \comp P_{\vx_k}^\dagger] \\
        &=  \lim_{k \to \infty} \lim_{i \to \infty} \E_{P_{\vx_k}\mu_i}[L \comp P_{\vx_k}^\dagger] \\
        &=  \lim_{k \to \infty} \E_{P_{\vx_k}\mu}[L \comp P_{\vx_k}^\dagger] \\
        &= \E_{\mu}[L]
    \end{align*}
    where the interchange of limits is justified by the aforementioned uniformity of convergence.
    Since $L$ was arbitrary, this shows that $\mu_i \weakto \mu$.
\end{proof}

A lemma that we will need later says that, if $(\mu_i)_{i=1}^\infty \sub \mathcal{P}$ are H\"older $L^{p,q}$-equicontinuous for some $p > 0$ and $q > 1$, then finite-dimensional distributions converge weakly in a uniform way if their inputs converge.

\begin{lemma} \label{lem:Holder_uniform_weak_convergence-fdds}
    Suppose that $(\mu_i)_{i=1}^\infty \sub \mathcal{P}$ are H\"older $L^{p,q}$-equicontinuous for some $p > 0$ and $q > 1$.
    For some $n \in \N$, let $(\vx_k)_{k \ge 1} \sub [0, 1]^n$ be convergent to some $\vx \in [0, 1]^n$.
    Then, for any $L\colon \R^n \to \R$ continuous and bounded,
    \begin{equation}
        \lim_{k \to \infty} \sup_{i \ge 1}\, \abs{
            \E_{P_{\vx_k} \mu_i}[L] - \E_{P_\vx \mu_i}[L]
        }
        = 0.
    \end{equation}
\end{lemma}
\begin{proof}
    Let $\e > 0$.
    Then there exists a $\delta > 0$ such that $\abs{L(\vy) - L(\vy')} < \e$ whenever $\norm{\vy - \vy'}_\infty < \delta$.
    Consider the event $A_\delta^k = \set{\norm{P_{\vx_k} f - P_{\vx} f}_\infty < \delta}$.
    Then estimate
    \begin{equation}
        \abs{
            \E_{\mu_i}[L \comp P_{\vx_k}]
            - \E_{\mu_i}[L \comp P_{\vx}]
        }
        \le
            \e + \norm{L}_\infty \mu_i((A^k_\delta)^\c)
        \le
            \e + \norm{L}_\infty \sup_{i \ge 1}\, \mu_i((A^k_\delta)^\c),
    \end{equation}
    and use \cref{lem:modulus_continuity} to take $k \to \infty$ and conclude.
\end{proof}

\end{document}
